# Supplementary material for: Assessing the Performances of CASPT2 and NEVPT2 for Vertical Excitation Energies
Source: arXiv:2111.15386 source file (2022-03-08)
Supplement: Supplementary file 1 [file Bench-CASPT2-SI-rev.pdf]

# Assessing the Performance of CASPT2 and NEVPT2 for Vertical Excitation Energies Supporting Information

Rudraditya Sarkar,[†] Pierre-François Loos,[‡] Martial Boggio-Pasqua,[*,‡] and Denis Jacquemin[*,†]

†*Laboratoire CEISAM - UMR CNRS 6230, Université de Nantes, 2 Rue de la Houssinière, BP 92208, 44322 Nantes Cedex 3, France*

‡*Laboratoire de Chimie et Physique Quantiques, CNRS et Université Toulouse III - Paul Sabatier, 118 route de Narbonne, 31062 Toulouse, France*

E-mail: martial.boggio@irsamc.ups-tlse.fr; Denis.Jacquemin@univ-nantes.fr

# S1 Active Spaces

In the following Tables, the vertical transition energies (VTEs) obtained with state-averaged CASSCF, state-specific CASPT2 using a level shift of 0.30 a.u. with or without an IPEA shift of 0.25 a.u., as well as the strongly-contracted (SC) and partially-contracted (PC) NEVPT2 methods are given for acetaldehyde, cyclopropene, diazomethane, formamide, ketene, nitrosomethane, streptocyanine-C1, and imidazole, together with a description of the respective active spaces. The composition of the active space is specified in terms of number of active orbitals per irreducible representation. The state-averaging procedure used is also described in terms of number of states per irreducible representation. We also provide the SA-CASSCF VTEs corresponding to the underlying reference calculation. Note that, for all calculations, the ground state is systematically included in the state averaging procedure even if it does not belong to the same irreducible representation. The cartesian coordinates for each compound detailed below can be found in the SI of a previous work.[1] For the active space description of the other molecules treated in the main text, please see the SI of our previous works.[2,3]

Table S1: VTEs (in eV) obtained at the CASSCF, CASPT2(IPEA), CASPT2(NOIPEA) and NEVPT2 levels of theory using the *aug*-cc-pVTZ basis set for acetaldehyde.

| State | Active space | State average | CASSCF | CASPT2 | | NEVPT2 | |
|---|---|---|---|---|---|---|---|
| | $(a', a'')$ | $(A', A'')$ | | IPEA | NOIPEA | PC | SC |
| $^1A''(\text{V}; n \to \pi^\star)$ | (3,2) | (1,1) | 4.62[a] | 4.35[a] | 4.13[a] | 4.39[a] | 4.42[a] |
| $^3A''(\text{V}; n \to \pi^\star)$ | (3,2) | (1,1) | 4.28[a] | 3.94[a] | 3.71[a] | 4.00[a] | 4.03[a] |

[a]Reference $(6e, 5o)$ active space including valence $n_O$, $\pi_{\text{CO}}$, $\sigma_{\text{CO}}$ and $\pi^\star_{\text{CO}}$, $\sigma^\star_{\text{CO}}$ orbitals.

Table S2: VTEs (in eV) obtained at the CASSCF, CASPT2(IPEA), CASPT2(NOIPEA) and NEVPT2 levels of theory using the *aug*-cc-pVTZ basis set for cyclopropene.

| State | Active space | State average | CASSCF | CASPT2 | | NEVPT2 | |
|---|---|---|---|---|---|---|---|
| | $(a_1, b_1, b_2, a_2)$ | $(A_1, B_1, B_2, A_2)$ | | IPEA | NOIPEA | PC | SC |
| $^1B_1(\mathrm{V}; \sigma \rightarrow \pi^\star)$ | (3,1,3,1) | (1,1,0,0) | 7.48[a] | 6.86[a] | 6.58[a] | 6.80[a] | 6.91[a] |
| $^1B_2(\mathrm{V}; \pi \rightarrow \pi^\star)$ | (3,1,3,1) | (1,0,1,0) | 7.47[a] | 6.89[a] | 6.47[a] | 6.83[a] | 6.95[a] |
| $^3B_2(\mathrm{V}; \pi \rightarrow \pi^\star)$ | (3,1,3,1) | (1,0,1,0) | 4.60[a] | 4.47[a] | 4.27[a] | 4.51[a] | 4.53[a] |
| $^3B_1(\mathrm{V}; \sigma \rightarrow \pi^\star)$ | (3,1,3,1) | (1,1,0,0) | 7.08[a] | 6.56[a] | 6.32[a] | 6.52[a] | 6.61[a] |

[a]Reference $(8e, 8o)$ active space including valence $\pi_{\mathrm{CC}}$, $\sigma_{\mathrm{CC}}$ and $\pi^\star_{\mathrm{CC}}$, $\sigma^\star_{\mathrm{CC}}$ orbitals.

Table S3: VTEs (in eV) obtained at the from CASSCF, CASPT2(IPEA), CASPT2(NOIPEA) and NEVPT2 levels of theory using the *aug*-cc-pVTZ basis set for diazomethane. [F] indicates the calculation of emission from the lowest $S_1$ geometry, i.e., a vertical fluorescence.

| State | Active space | State average | CASSCF | CASPT2 | | NEVPT2 | |
|---|---|---|---|---|---|---|---|
| | $(a_1, b_1, b_2, a_2)$ | $(A_1, B_1, B_2, A_2)$ | | IPEA | NOIPEA | PC | SC |
| $^1A_2$(V; $\pi \rightarrow \pi^\star$) | (4,3,2,0) | (1,0,0,1) | $3.27^a$ | $3.13^a$ | $2.92^a$ | $3.09^a$ | $3.13^a$ |
| $^1B_1$(R; $\pi \rightarrow 3s$) | (5,3,2,0) | (1,1,0,0) | $4.59^b$ | $5.50^b$ | $5.30^b$ | $5.63^b$ | $5.57^b$ |
| $^1A_1$(V; $\pi \rightarrow \pi^\star$) | (4,3,2,0) | (2,0,0,0) | $7.17^a$ | $6.43^a$ | $5.41^a$ | $6.17^a$ | $6.63^a$ |
| | (4,4,2,0) | (3,0,0,0) | $5.65^c$ | $6.21^c$ | $5.92^c$ | $6.23^c$ | $6.28^c$ |
| $^1A_1$(R; $\pi \rightarrow 3p$) | (4,4,2,0) | (3,0,0,0) | $8.46^c$ | $7.80^c$ | $7.14^c$ | $7.64^c$ | $7.97^c$ |
| $^3A_2$(V; $\pi \rightarrow \pi^\star$) | (4,3,2,0) | (1,0,0,1) | $3.02^a$ | $2.87^a$ | $2.67^a$ | $2.83^a$ | $2.88^a$ |
| $^3A_1$(V; $\pi \rightarrow \pi^\star$) | (4,3,2,0) | (2,0,0,0) | $4.27^a$ | $4.10^a$ | $3.88^a$ | $4.07^a$ | $4.12^a$ |
| | (4,4,2,0) | (3,0,0,0) | $4.26^c$ | $4.16^c$ | $3.90^c$ | $4.08^c$ | $4.14^c$ |
| $^3B_1$(R; $\pi \rightarrow 3s$) | (5,3,2,0) | (1,1,0,0) | $4.45^b$ | $5.34^b$ | $5.15^b$ | $5.48^b$ | $5.42^b$ |
| $^3A_1$(R; $\pi \rightarrow 3p$) | (4,4,2,0) | (3,0,0,0) | $6.34^c$ | $7.00^c$ | $6.76^c$ | $7.01^c$ | $7.02^c$ |
| $^1A''$[F](V; $\pi \rightarrow \pi^\star$) | ($a'$:6, $a''$:3) | ($A'$:1, $A''$:1) | $0.72^a$ | $0.69^a$ | $0.52^a$ | $0.66^a$ | $0.68^a$ |

[a]Reference $(10e, 9o)$ active space including valence $\pi$, $\sigma_{\mathrm{CN}}$, $\sigma_{\mathrm{NN}}$ and $\sigma^\star_{\mathrm{CN}}$, $\sigma^\star_{\mathrm{NN}}$ orbitals. [b]Reference $(10e, 10o)$ active space including valence $\pi$, $\sigma_{\mathrm{CN}}$, $\sigma_{\mathrm{NN}}$ and $\sigma^\star_{\mathrm{CN}}$, $\sigma^\star_{\mathrm{NN}}$, Rydberg $3s$ orbitals. [c]Reference $(10e, 10o)$ active space including valence $\pi$, $\sigma_{\mathrm{CN}}$, $\sigma_{\mathrm{NN}}$ and $\sigma^\star_{\mathrm{CN}}$, $\sigma^\star_{\mathrm{NN}}$, Rydberg $3p$ orbitals.

Table S4: VTEs (in eV) obtained at the CASSCF, CASPT2(IPEA), CASPT2(NOIPEA) and NEVPT2 levels of theory using the *aug*-cc-pVTZ basis set for formamide.

| State | Active space | State average | CASSCF | CASPT2 | | NEVPT2 | |
|---|---|---|---|---|---|---|---|
| | $(a', a'')$ | $(A', A'')$ | | IPEA | NOIPEA | PC | SC |
| $^1A''(\mathrm{V}; n \to \pi^\star)$ | (5,3) | (1,1) | $5.95^a$ | $5.66^a$ | $5.45^a$ | $5.71^a$ | $5.73^a$ |
| $^1A'(\mathrm{R}; n \to 3s)$ | (7,3) | (4,0) | $6.17^b$ | $6.80^b$ | $6.64^b$ | $6.98^b$ | $6.92^b$ |
| $^1A'(\mathrm{V}; \pi \to \pi^\star)$ | (4,3) | (2,0) | $8.34^c$ | $7.60^c$ | $7.06^c$ | $7.53^c$ | $7.84^c$ |
| | (7,3) | (4,0) | $8.80^b$ | $7.88^b$ | $7.13^b$ | $7.64^b$ | $8.11^b$ |
| $^1A'(\mathrm{R}; n \to 3p)$ | (7,3) | (4,0) | $6.74^b$ | $7.45^b$ | $7.32^b$ | $7.64^b$ | $7.57^b$ |
| $^3A''(\mathrm{V}; n \to \pi^\star)$ | (5,3) | (1,1) | $5.89^a$ | $5.36^a$ | $5.16^a$ | $5.38^a$ | $5.44^a$ |
| $^3A'(\mathrm{V}; \pi \to \pi^\star)$ | (4,3) | (2,0) | $6.10^c$ | $5.88^c$ | $5.62^c$ | $5.90^c$ | $5.98^c$ |

[a]Reference $(10e, 8o)$ active space including valence $\pi$, $n_\mathrm{O}$ $\sigma_\mathrm{CN}$, $\sigma_\mathrm{CO}$ and $\sigma^\star_\mathrm{CN}$, $\sigma^\star_\mathrm{CO}$ orbitals. [b]Reference $(10e, 10o)$ active space including valence $\pi$, $n_\mathrm{O}$ $\sigma_\mathrm{CN}$, $\sigma_\mathrm{CO}$ and $\sigma^\star_\mathrm{CN}$, $\sigma^\star_\mathrm{CO}$, Rydberg $3s$, Rydberg $3p$ orbitals. [c]Reference $(8e, 7o)$ active space including valence $\pi$, $\sigma_\mathrm{CN}$, $\sigma_\mathrm{CO}$ and $\sigma^\star_\mathrm{CN}$, $\sigma^\star_\mathrm{CO}$ orbitals.

Table S5: VTEs (in eV) obtained at the CASSCF, CASPT2(IPEA), CASPT2(NOIPEA) and NEVPT2 levels of theory using the *aug*-cc-pVTZ basis set for ketene. [F] indicates the calculation of emission from the lowest $S_1$ geometry, i.e., a vertical fluorescence.

| State | Active space | State average | CASSCF | CASPT2 | | NEVPT2 | |
|---|---|---|---|---|---|---|---|
| | $(a_1, b_1, b_2, a_2)$ | $(A_1, B_1, B_2, A_2)$ | | IPEA | NOIPEA | PC | SC |
| $^1A_2(\text{V}; \pi \rightarrow \pi^\star)$ | (4,3,2,0) | (1,0,0,1) | 3.98[a] | 3.92[a] | 3.70[a] | 3.93[a] | 3.97[a] |
| | (4,3,3,0) | (1,0,0,2) | 4.09[b] | 3.97[b] | 3.70[b] | 3.96[b] | 4.03[b] |
| $^1B_1(\text{R}; \pi \rightarrow 3s)$ | (5,3,2,0) | (1,1,0,0) | 5.22[c] | 5.99[c] | 5.79[c] | 6.09[c] | 6.07[c] |
| $^1A_2(\text{R}; \pi \rightarrow 3p)$ | (4,3,3,0) | (1,0,0,2) | 6.38[b] | 7.25[b] | 7.05[b] | 7.28[b] | 7.26[b] |
| $^3A_2(\text{V}; \pi \rightarrow \pi^\star)$ | (4,3,2,0) | (1,0,0,1) | 3.92[a] | 3.81[a] | 3.59[a] | 3.80[a] | 3.85[a] |
| | (4,3,3,0) | (1,0,0,2) | 4.04[b] | 3.87[b] | 3.60[b] | 3.83[b] | 3.91[b] |
| $^3A_1(\text{V}; \pi \rightarrow \pi^\star)$ | (4,3,2,0) | (2,0,0,0) | 5.79[a] | 5.65[a] | 5.43[a] | 5.65[a] | 5.69[a] |
| $^3B_1(\text{R}; \pi \rightarrow 3s)$ | (5,3,2,0) | (1,1,0,0) | 5.05[c] | 5.79[c] | 5.60[c] | 5.89[c] | 5.87[c] |
| $^3A_2(\text{R}; \pi \rightarrow 3p)$ | (4,3,3,0) | (1,0,0,2) | 6.35[b] | 7.21[b] | 7.01[b] | 7.24[b] | 7.22[b] |
| $^1A^{''}[\text{F}](\text{V}; \pi \rightarrow \pi^\star)$ | $(a^{'}$:6, $a^{''}$:3) | $(A^{'}$:1, $A^{''}$:1) | 0.95[a] | 1.05[a] | 0.88[a] | 1.02[a] | 1.04[a] |

[a]Reference $(10e, 9o)$ active space including valence $\pi$, $\sigma_{CC}$, $\sigma_{CO}$ and $\sigma^\star_{CC}$, $\sigma^\star_{CO}$ orbitals. [b]Reference $(10e, 10o)$ active space including valence $\pi$, $\sigma_{CC}$, $\sigma_{CO}$ and $\sigma^\star_{CC}$, $\sigma^\star_{CO}$, Rydberg $3p$ orbitals. [c]Reference $(10e, 10o)$ active space including valence $\pi$, $\sigma_{CC}$, $\sigma_{CO}$ and $\sigma^\star_{CC}$, $\sigma^\star_{CO}$, Rydberg $3s$ orbitals.

Table S6: VTEs (in eV) obtained at the CASSCF, CASPT2(IPEA), CASPT2(NOIPEA) and NEVPT2 levels of theory using the *aug*-cc-pVTZ basis set for nitrosomethane. [F] indicates the calculation of emission from the lowest $S_1$ geometry, i.e., a vertical fluorescence.

| State | Active space | State average | CASSCF | CASPT2 | | NEVPT2 | |
|---|---|---|---|---|---|---|---|
| | $(a', a'')$ | $(A', A'')$ | | IPEA | NOIPEA | PC | SC |
| $^1A''(\mathrm{V}; n \to \pi^\star)$ | (4,2) | (1,1) | 2.12[a] | 1.84[a] | 1.60[a] | 1.91[a] | 1.94[a] |
| $^1A'(\mathrm{V}; n, n \to \pi^\star, \pi^\star)$ | (4,2) | (2,0) | 4.74[a] | 4.69[a] | 4.67[a] | 4.73[a] | 4.73[a] |
| | (5,2) | (3,0) | 4.71[b] | 4.68[b] | 4.67[b] | 4.77[b] | 4.75[b] |
| $^1A'(\mathrm{R}; n \to 3s)$ | (5,2) | (3,0) | 5.87[b] | 6.32[b] | 6.07[b] | 6.38[b] | 6.38[b] |
| $^3A''(\mathrm{V}; n \to \pi^\star)$ | (4,2) | (1,1) | 1.31[a] | 1.00[a] | 0.75[a] | 1.08[a] | 1.13[a] |
| $^3A'(\mathrm{V}; \pi \to \pi^\star)$ | (2,2) | (2,0) | 5.52[c] | 5.52[c] | 5.37[c] | 5.54[c] | 5.54[c] |
| $^1A''$[F]$(\mathrm{V}; n \to \pi^\star)$ | (4,2) | (1,1) | 1.83[a] | 1.55[a] | 1.32[a] | 1.62[a] | 1.66[a] |

[a]Reference $(8e, 6o)$ active space including valence $n_{\mathrm{O}}$, $n_{\mathrm{N}}$, $\pi_{\mathrm{NO}}$, $\sigma_{\mathrm{NO}}$ and $\sigma^\star_{\mathrm{NO}}$, $\pi^\star_{\mathrm{NO}}$ orbitals. [b]Reference $(8e, 7o)$ active space including valence $n_{\mathrm{O}}$, $n_{\mathrm{N}}$, $\pi_{\mathrm{NO}}$, $\sigma_{\mathrm{NO}}$ and $\sigma^\star_{\mathrm{NO}}$, $\pi^\star_{\mathrm{NO}}$, Rydberg $3s$ orbitals. [c]Reference $(4e, 4o)$ active space including valence $\pi_{\mathrm{NO}}$, $\sigma_{\mathrm{NO}}$ and $\sigma^\star_{\mathrm{NO}}$, $\pi^\star_{\mathrm{NO}}$ orbitals.

Table S7: VTEs (in eV) obtained at the CASSCF, CASPT2(IPEA), CASPT2(NOIPEA) and NEVPT2 levels of theory using the *aug*-cc-pVTZ basis set for streptocyanine-C1.

| State | Active space | State average | CASSCF | CASPT2 | | NEVPT2 | |
|---|---|---|---|---|---|---|---|
| | $(a_1, b_1, b_2, a_2)$ | $(A_1, B_1, B_2, A_2)$ | | IPEA | NOIPEA | PC | SC |
| $^1B_2(\mathrm{V}; \pi \rightarrow \pi^\star)$ | (2,2,2,1) | (1,0,1,0) | 7.82[a] | 7.17[a] | 6.76[a] | 7.13[a] | 7.34[a] |
| $^3B_2(\mathrm{V}; \pi \rightarrow \pi^\star)$ | (2,2,2,1) | (1,0,1,0) | 5.86[a] | 5.49[a] | 5.22[a] | 5.52[a] | 5.62[a] |

[a]Reference $(8e, 7o)$ active space including valence $\pi$, two $\sigma_{CN}$ and two $\sigma^\star_{CN}$ orbitals.

Table S8: VTEs (in eV) obtained at the CASSCF, CASPT2(IPEA), CASPT2(NOIPEA) and NEVPT2 levels of theory using the *aug*-cc-pVTZ basis set for imidazole.

| State | Active space | State average | CASSCF | CASPT2 | | NEVPT2 | |
|---|---|---|---|---|---|---|---|
| | $(a', a'')$ | $(A', A'')$ | | IPEA | NOIPEA | PC | SC |
| $^1A''(\mathrm{R}; \pi \rightarrow 3s)$ | (2,5) | (1,3) | $5.04^a$ | $5.88^a$ | $5.66^a$ | $5.93^a$ | $5.92^a$ |
| | (4,6) | (1,7) | $4.70^b$ | $5.75^b$ | $5.62^b$ | $6.02^b$ | $5.98^b$ |
| $^1A'(\mathrm{R}; \pi \rightarrow 3p)$ | (0,9) | (3,0) | $6.18^c$ | $6.69^c$ | $6.45^c$ | $6.73^c$ | $6.77^c$ |
| $^1A''(\mathrm{R}; \pi \rightarrow 3p)$ | (4,6) | (1,7) | $5.43^b$ | $6.57^b$ | $6.47^b$ | $6.83^b$ | $6.80^b$ |
| $^1A''(\mathrm{V}; n \rightarrow \pi^\star)$ | (2,5) | (1,3) | $7.13^a$ | $6.94^a$ | $6.57^a$ | $6.96^a$ | $7.01^a$ |
| | (4,6) | (1,7) | $7.34^b$ | $7.06^b$ | $6.62^b$ | $7.00^b$ | $7.07^b$ |
| $^1A'(\mathrm{V}; \pi \rightarrow \pi^\star)$ | (0,9) | (3,0) | $6.73^c$ | $6.88^c$ | $6.46^c$ | $7.00^c$ | $7.06^c$ |
| $^1A'(\mathrm{R}; n \rightarrow 3s)$ | (2,5) | (2,0) | $6.36^a$ | $7.10^a$ | $6.91^a$ | $7.20^a$ | $7.20^a$ |
| $^3A'(\mathrm{V}; \pi \rightarrow \pi^\star)$ | (0,9) | (3,0) | $4.55^c$ | $4.78^c$ | $4.53^c$ | $4.86^c$ | $4.88^c$ |
| $^3A''(\mathrm{R}; \pi \rightarrow 3s)$ | (2,5) | (1,3) | $5.03^a$ | $5.86^a$ | $5.63^a$ | $5.91^a$ | $5.90^a$ |
| $^3A'(\mathrm{V}; \pi \rightarrow \pi^\star)$ | (0,9) | (3,0) | $5.69^c$ | $5.85^c$ | $5.48^c$ | $5.91^c$ | $5.96^c$ |
| $^3A''(\mathrm{V}; n \rightarrow \pi^\star)$ | (2,5) | (1,3) | $6.58^a$ | $6.44^a$ | $6.10^a$ | $6.48^a$ | $6.51^a$ |

[a]Reference $(8e, 7o)$ active space including valence $\pi$, $n_\mathrm{N}$, and Rydberg $3s$ orbitals. [b]Reference $(8e, 10o)$ active space including valence $\pi$, $n_\mathrm{N}$, Rydberg $3s$ and three Rydberg $3p$ orbitals. [c]Reference $(6e, 9o)$ active space including valence $\pi$ and four Rydberg $3p$ orbitals.

# S2 Corrected data for cyanoacetylene, isobutene and triazine

Below is an updated Table S16 of Ref. 3 in which a misprint has been corrected regarding the active space description.

Table S9: NEVPT2/aug-cc-pVTZ vertical transition energies (in eV) of cyanoacetylene.

| State | Active space $(a_1, b_1, b_2, a_2)$ | State average $(A_1, B_1, B_2, A_2)$ | CASSCF[a] | NEVPT2[a] |
|---|---|---|---|---|
| $^1\Sigma^-(\mathrm{V}; \pi \to \pi^\star)$ | (0,4,4,0) | (1,0,0,1) | 6.54 | 5.78 |
| $^1\Delta(\mathrm{V}; \pi \to \pi^\star)$ | (0,4,4,0) | (2,0,0,1) | 6.80 | 6.10 |
| $^3\Sigma^+(\mathrm{V}; \pi \to \pi^\star)$ | (0,4,4,0) | (2,0,0,0) | 4.86 | 4.45 |
| $^3\Delta(\mathrm{V}; \pi \to \pi^\star)$ | (0,4,4,0) | (2,0,0,1) | 5.64 | 5.19 |
| $^1A''[\mathrm{F}](\mathrm{V}; \pi \to \pi^\star)$ | ($a'$:4,$a''$:4) | ($A'$:1,$A''$:1) | 4.30 | 3.50 |

[a] All calculations using a full valence $\pi$ active space of (8e,8o).

Below is an updated Table S26 of Ref. 3 in which a misprint has been corrected regarding the CASSCF energy of the lowest singlet state.

Table S10: NEVPT2/aug-cc-pVTZ vertical transition energies (in eV) of isobutene.

| State | Active space $(a_1, b_1, b_2, a_2)$ | State average $(A_1, B_1, B_2, A_2)$ | CASSCF | NEVPT2 |
|---|---|---|---|---|
| $^1B_1(\mathrm{R}; \pi \to 3s)$ | (3,2,0,0) | (1,1,0,0) | 6.21[a] | 6.63[a] |
| $^1A_1(\mathrm{R}; \pi \to 3p)$ | (2,3,0,0) | (2,0,0,0) | 6.90[b] | 7.20[b] |
| $^3A_1(\mathrm{V}; \pi \to \pi^\star)$ | (2,2,0,0) | (2,0,0,0) | 4.66[c] | 4.61[c] |

[a] Reference $(4e, 5o)$ active space including valence $\pi$, $\sigma_{\mathrm{CC}}$, $\sigma^*_{\mathrm{CC}}$ and $3s$ orbitals. [b] Reference $(4e, 5o)$ active space including valence $\pi$, $\sigma_{\mathrm{CC}}$, $\sigma^*_{\mathrm{CC}}$ and $3p_x$ orbitals. [c] Reference $(4e, 4o)$ active space including valence $\pi$, $\sigma_{\mathrm{CC}}$ and $\sigma^*_{\mathrm{CC}}$ orbitals.

Below is an updated Table S38 of Ref. 3 in which a misprint has been corrected regarding the CASSCF transition energy of the Rydberg state.

Table S11: NEVPT2/aug-cc-pVTZ vertical transition energies (in eV) of triazine.

| State | Active space $(a_1, b_1, b_2, a_2)$ | State average $(A_1, B_1, B_2, A_2)$ | CASSCF | NEVPT2 |
|---|---|---|---|---|
| $^1A_1''(\text{V}; n \to \pi^\star)$ | (2,4,1,2) | (1,2,0,2) | $5.88^a$ | $4.61^a$ |
| $^1A_2''(\text{V}; n \to \pi^\star)$ | (2,4,1,2) | (1,1,0,0) | $5.14^a$ | $4.89^a$ |
| $^1E''(\text{V}; n \to \pi^\star)$ | (2,4,1,2) | (1,2,0,2) | $5.51^a$ | $4.88^a$ |
| $^1A_2'(\text{V}; \pi \to \pi^\star)$ | (0,6,0,3) | (1,0,1,0) | $5.55^d$ | $6.10^b$,$6.15^c$,$5.95^d$ |
| $^1A_1'(\text{V}; \pi \to \pi^\star)$ | (0,6,0,3) | (2,0,0,0) | $8.20^d$ | $7.06^b$,$7.30^d$ |
| $^1E'(\text{R}; n \to 3s)$ | (3,4,1,2) | (2,0,2,0) | $7.40^c$ | $7.45^c$ |
| $^1E''(\text{V}; n \to \pi^\star)$ | (2,4,1,2) | (1,1,0,1) | $8.26^a$ | $7.98^a$ |
| $^1E'(\text{V}; \pi \to \pi^\star)$ | (0,6,0,3) | (4,0,3,0) | $10.03^d$ | $7.74^b$,$8.34^d$ |
| $^3A_2''(\text{V}; n \to \pi^\star)$ | (2,4,1,2) | (1,1,0,0) | $4.74^a$ | $4.51^a$ |
| $^3E''(\text{V}; n \to \pi^\star)$ | (2,4,1,2) | (1,2,0,2) | $5.14^a$ | $4.61^a$ |
| $^3A_1''(\text{V}; n \to \pi^\star)$ | (2,4,1,2) | (1,2,0,2) | $5.88^a$ | $4.71^a$ |
| $^3A_1'(\text{V}; \pi \to \pi^\star)$ | (0,6,0,3) | (2,0,0,0) | $4.46^d$ | $5.20^b$,$5.05^d$ |
| $^3E'(\text{V}; \pi \to \pi^\star)$ | (0,6,0,3) | (3,0,1,0) | $5.57^d$ | $5.83^b$,$5.73^d$ |
| $^3A_2'(\text{V}; (\pi \to \pi^\star)$ | (0,6,0,3) | (1,0,1,0) | $7.70^d$ | $5.83^b$,$6.36^d$ |

[a]Reference $(12e, 9o)$ active space including valence $\pi$ and $n_\text{N}$ orbitals. [b]Reference $(6e, 6o)$ active space including valence $\pi$ orbitals. [c]Reference $(12e, 10o)$ active space including valence $\pi$, $n_\text{N}$ and $3s$ orbitals. [d]Reference $(6e, 9o)$ active space including valence $\pi$ and three $3p_x$ orbitals.

# S3 TBEs for imidazole's singlet ESs

Below, we provide a corrected and extended version of Table 6 of Ref. 3 with additional transitions for singlet ESs (six transitions here rather than four in the original work).

Table S12: Vertical transition energies (in eV) of imidazole.

| | 6-31+G(d) | | *aug*-cc-pVDZ | | *aug*-cc-pVTZ | *aug*-cc-pVTZ |
|---|---|---|---|---|---|---|
| State | CC3 | CCSDT | CC3 | CCSDT | CC3 | TBE |
| $^1A''(\pi \to 3s)$ | 5.77 | 5.77 | 5.60 | 5.60 | 5.70 | 5.70[b] |
| $^1A'(\pi \to 3p)^a$ | 6.51 | 6.51 | 6.43 | 6.43 | 6.41 | 6.41[b] |
| $^1A''(n \to 3p)$ | 6.66 | 6.66 | 6.42 | 6.42 | 6.50 | 6.50[b] |
| $^1A''(n \to \pi^\star)$ | 6.91 | 6.89 | 6.79 | 6.77 | 6.73 | 6.71[b] |
| $^1A'(\pi \to \pi^\star)^a$ | 7.04 | 7.02 | 6.89 | 6.89 | 6.87 | 6.86[b] |
| $^1A'(n \to 3s)$ | 7.12 | 7.12 | 6.93 | 6.92 | 7.02 | 7.00[b] |
| $^3A'(\pi \to \pi^\star)$ | 4.83 | 4.81 | 4.78 | | 4.75 | 4.74[c] |
| $^3A''(\pi \to 3s)$ | 5.72 | 5.72 | 5.57 | 5.56 | 5.67 | 5.66[b] |
| $^3A'(\pi \to \pi^\star)$ | 5.88 | 5.88 | 5.78 | | 5.74 | 5.74[c] |
| $^3A''(n \to \pi^\star)$ | 6.48 | 6.46 | 6.37 | 6.35 | 6.33 | 6.31[b] |

[a]Strong valence/Rydberg mixing; [b]CC3/*aug*-cc-pVTZ result corrected by the difference between CCSDT/*aug*-cc-pVDZ and CC3/*aug*-cc-pVTZ values; [b]CC3/*aug*-cc-pVTZ result corrected by the difference between CCSDT/6-31+G(d) and CC3/6-31+G(d) values.

# S4 Additional Data

Table S13: Comparisons between theoretical best estimates (TBEs) obtained with *aug*-cc-pVTZ and VTEs obtained at the CASSCF (CAS) and SC-NEVPT2 (SC-NEV) levels of theory. All values are in eV. Italics are used for the *unsafe* TBEs.

| Compound | State | TBE | CAS | SCNEV |
|---|---|---|---|---|
| Acetaldehyde | $^1A''(\mathrm{V}; n \rightarrow \pi^\star)$ | 4.31 | 4.62 | 4.42 |
| | $^3A''(\mathrm{V}; n \rightarrow \pi^\star)$ | 3.97 | 4.28 | 4.03 |
| Acetone | $^1A_2(\mathrm{V}; n \rightarrow \pi^\star)$ | 4.47 | 4.77 | 4.50 |
| | $^1B_2(\mathrm{R}; n \rightarrow 3s)$ | 6.46 | 5.50 | 6.70 |
| | $^1A_2(\mathrm{R}; n \rightarrow 3p)$ | 7.47 | 7.46 | 7.71 |
| | $^1A_1(\mathrm{R}; n \rightarrow 3p)$ | 7.51 | 7.03 | 7.75 |
| | $^1B_2(\mathrm{R}; n \rightarrow 3p)$ | 7.62 | 6.44 | 7.80 |
| | $^3A_2(\mathrm{V}; n \rightarrow \pi^\star)$ | 4.13 | 4.47 | 4.22 |
| | $^3A_1(\mathrm{V}; \pi \rightarrow \pi^\star)$ | 6.25 | 6.22 | 6.28 |
| Acrolein | $^1A''(\mathrm{V}; n \rightarrow \pi^\star)$ | 3.78 | 4.02 | 3.78 |
| | $^1A'(\mathrm{V}; \pi \rightarrow \pi^\star)$ | 6.69 | 8.24 | 7.02 |
| | $^1A''(\mathrm{V}; n \rightarrow \pi^\star)$ | *6.72* | 7.63 | 7.30 |
| | $^1A'(\mathrm{R}; n \rightarrow 3s)$ | 7.08 | 6.98 | 7.14 |
| | $^1A'(\mathrm{V}; \pi \rightarrow \pi^\star)$[a] | 7.87 | 8.86 | 8.05 |
| | $^3A''(\mathrm{V}; n \rightarrow \pi^\star)$ | 3.51 | 3.86 | 3.36 |
| | $^3A'(\mathrm{V}; \pi \rightarrow \pi^\star)$ | 3.94 | 4.31 | 4.02 |
| | $^3A'(\mathrm{V}; \pi \rightarrow \pi^\star)$ | 6.18 | 6.76 | 6.34 |
| | $^3A''(\mathrm{V}; n \rightarrow \pi^\star)$ | *6.54* | 7.47 | 6.83 |
| Benzene | $^1B_{2u}(\mathrm{V}; \pi \rightarrow \pi^\star)$ | 5.06 | 4.98 | 5.35 |
| | $^1B_{1u}(\mathrm{V}; \pi \rightarrow \pi^\star)$ | 6.45 | 7.27 | 6.48 |
| | $^1E_{1g}(\mathrm{R}; \pi \rightarrow 3s)$ | *6.52* | 5.90 | 6.76 |
| | $^1A_{2u}(\mathrm{R}; \pi \rightarrow 3p)$ | 7.08 | 6.14 | 7.40 |
| | $^1E_{2u}(\mathrm{R}; \pi \rightarrow 3p)$ | 7.15 | 6.21 | 7.45 |
| | $^1E_{2g}(\mathrm{V}; \pi \rightarrow \pi^\star)$[a] | 8.28 | 8.10 | 8.55 |
| | $^3B_{1u}(\mathrm{V}; \pi \rightarrow \pi^\star)$ | 4.16 | 3.85 | 4.33 |
| | $^3E_{1u}(\mathrm{V}; \pi \rightarrow \pi^\star)$ | 4.85 | 4.85 | 4.94 |
| | $^3B_{2u}(\mathrm{V}; \pi \rightarrow \pi^\star)$ | 5.81 | 6.75 | 5.59 |
| Butadiene | $^1B_u(\mathrm{V}; \pi \rightarrow \pi^\star)$ | 6.22 | 6.65 | 6.72 |
| | $^1B_g(\mathrm{R}; \pi \rightarrow 3s)$ | 6.33 | 5.94 | 6.48 |
| | $^1A_g(\mathrm{V}; \pi \rightarrow \pi^\star)$[a] | 6.50 | 6.99 | 6.78 |
| | $^1A_u(\mathrm{R}; \pi \rightarrow 3p)$ | 6.64 | 5.95 | 6.81 |
| | $^1A_u(\mathrm{R}; \pi \rightarrow 3p)$ | 6.80 | 6.12 | 7.00 |
| | $^1B_u(\mathrm{R}; \pi \rightarrow 3p)$ | 7.68 | 7.93 | 7.53 |
| | $^3B_u(\mathrm{V}; \pi \rightarrow \pi^\star)$ | 3.36 | 3.55 | 3.43 |
| | $^3A_g(\mathrm{V}; \pi \rightarrow \pi^\star)$ | 5.20 | 5.52 | 5.36 |
| | $^3B_g(\mathrm{R}; \pi \rightarrow 3s)$ | 6.29 | 5.89 | 6.43 |
| Carbon trimer | $^1\Delta_g(\mathrm{V}; n, n \rightarrow \pi^\star, \pi^\star)$ | 5.22 | 4.98 | 5.21 |
| | $^1\Sigma_g^+(\mathrm{V}; n, n \rightarrow \pi^\star, \pi^\star)$ | 5.91 | 5.84 | 5.99 |
| Cyanoacetylene | $^1\Sigma^-(\mathrm{V}; \pi \rightarrow \pi^\star)$ | 5.80 | 6.54 | 5.83 |
| | $^1\Delta(\mathrm{V}; \pi \rightarrow \pi^\star)$ | 6.07 | 6.80 | 6.14 |
| | $^3\Sigma^+(\mathrm{V}; \pi \rightarrow \pi^\star)$ | 4.44 | 4.86 | 4.49 |
| | $^3\Delta(\mathrm{V}; \pi \rightarrow \pi^\star)$ | 5.21 | 5.64 | 5.23 |
| | $^1A''[\mathrm{F}](\mathrm{V}; \pi \rightarrow \pi^\star)$ | 3.54 | 4.30 | 3.55 |
| Cyanoformaldehyde | $^1A''(\mathrm{V}; n \rightarrow \pi^\star)$ | 3.81 | 4.02 | 4.01 |
| | $^1A''(\mathrm{V}; \pi \rightarrow \pi^\star)$ | 6.46 | 7.61 | 6.52 |
| | $^3A''(\mathrm{V}; n \rightarrow \pi^\star)$ | 3.44 | 3.52 | 3.59 |
| | $^3A'(\mathrm{V}; \pi \rightarrow \pi^\star)$ | 5.01 | 4.98 | 5.37 |
| Cyanogen | $^1\Sigma_u^-(\mathrm{V}; \pi \rightarrow \pi^\star)$ | 6.39 | 7.14 | 6.37 |
| | $^1\Delta_u(\mathrm{V}; \pi \rightarrow \pi^\star)$ | 6.66 | 7.46 | 6.71 |
| | $^3\Sigma_u^+(\mathrm{V}; \pi \rightarrow \pi^\star)$ | 4.91 | 5.28 | 4.92 |
| | $^1\Sigma_u^-[\mathrm{F}](\mathrm{V}; \pi \rightarrow \pi^\star)$ | 5.05 | 5.68 | 5.01 |
| Cyclopentadiene | $^1B_2(\mathrm{V}; \pi \rightarrow \pi^\star)$ | 5.56 | 6.71 | 5.71 |
| | $^1A_2(\mathrm{R}; \pi \rightarrow 3s)$ | 5.78 | 5.21 | 5.92 |
| | $^1B_1(\mathrm{R}; \pi \rightarrow 3p)$ | 6.41 | 6.08 | 6.43 |
| | $^1A_2(\mathrm{R}; \pi \rightarrow 3p)$ | 6.46 | 5.78 | 6.59 |
| | $^1B_2(\mathrm{R}; \pi \rightarrow 3p)$ | 6.56 | 6.16 | 6.62 |
| | $^1A_1(\mathrm{V}; \pi \rightarrow \pi^\star)$[a] | *6.52* | 6.49 | 6.78 |
| | $^3B_2(\mathrm{V}; \pi \rightarrow \pi^\star)$ | 3.31 | 3.26 | 3.42 |
| | $^3A_1(\mathrm{V}; \pi \rightarrow \pi^\star)$ | 5.11 | 4.92 | 5.31 |
| | $^3A_2(\mathrm{R}; \pi \rightarrow 3s)$ | 5.73 | 5.53 | 5.74 |
| | $^3B_1(\mathrm{R}; \pi \rightarrow 3p)$ | 6.36 | 6.05 | 6.41 |
| Cyclopropene | $^1B_1(\mathrm{V}; \sigma \rightarrow \pi^\star)$ | 6.68 | 7.48 | 6.91 |
| | $^1B_2(\mathrm{V}; \pi \rightarrow \pi^\star)$ | 6.79 | 7.47 | 6.95 |
| | $^3B_2(\mathrm{V}; \pi \rightarrow \pi^\star)$ | 4.38 | 4.60 | 4.53 |
| | $^3B_1(\mathrm{V}; \sigma \rightarrow \pi^\star)$ | 6.45 | 7.08 | 6.61 |
| Cyclopropenone | $^1B_1(\mathrm{V}; n \rightarrow \pi^\star)$ | 4.26 | 4.92 | 4.08 |
| | $^1A_2(\mathrm{V}; n \rightarrow \pi^\star)$ | 5.55 | 5.64 | 5.86 |
| | $^1B_2(\mathrm{R}; n \rightarrow 3s)$ | 6.34 | 5.68 | 6.47 |
| | $^1B_2(\mathrm{V}; \pi \rightarrow \pi^\star)$ | 6.54 | 6.40 | 6.82 |
| | $^1B_2(\mathrm{R}; n \rightarrow 3p)$ | 6.98 | 6.35 | 7.05 |
| | $^1A_1(\mathrm{R}; n \rightarrow 3p)$ | 7.02 | 6.84 | 7.29 |
| | $^1A_1(\mathrm{V}; \pi \rightarrow \pi^\star)$ | 8.28 | 10.42 | 8.81 |
| | $^3B_1(\mathrm{V}; n \rightarrow \pi^\star)$ | 3.93 | 4.72 | 3.55 |
| | $^3B_2(\mathrm{V}; \pi \rightarrow \pi^\star)$ | 4.88 | 4.39 | 5.07 |
| | $^3A_2(\mathrm{V}; n \rightarrow \pi^\star)$ | 5.35 | 5.40 | 5.60 |
| | $^3A_1(\mathrm{V}; \pi \rightarrow \pi^\star)$ | 6.79 | 6.59 | 7.17 |
| Cyclopropenethione | $^1A_2(\mathrm{V}; n \rightarrow \pi^\star)$ | 3.41 | 3.44 | 3.54 |
| | $^1B_1(\mathrm{V}; n \rightarrow \pi^\star)$ | 3.45 | 3.57 | 3.51 |
| | $^1B_2(\mathrm{V}; \pi \rightarrow \pi^\star)$ | 4.60 | 4.51 | 4.79 |
| | $^1B_2(\mathrm{R}; n \rightarrow 3s)$ | 5.34 | 4.59 | 5.34 |
| | $^1A_1(\mathrm{V}; \pi \rightarrow \pi^\star)$ | 5.46 | 6.46 | 5.72 |
| | $^1B_2(\mathrm{R}; n \rightarrow 3p)$ | 5.92 | 5.27 | 5.98 |
| | $^3A_2(\mathrm{V}; n \rightarrow \pi^\star)$ | 3.28 | 3.26 | 3.40 |
| | $^3B_1(\mathrm{V}; n \rightarrow \pi^\star)$ | 3.32 | 3.51 | 3.41 |
| | $^3B_2(\mathrm{V}; \pi \rightarrow \pi^\star)$ | 4.01 | 3.80 | 4.17 |
| | $^3A_1(\mathrm{V}; \pi \rightarrow \pi^\star)$ | 4.01 | 3.83 | 4.14 |
| Diacetylene | $^1\Sigma_u^-(\mathrm{V}; \pi \rightarrow \pi^\star)$ | 5.33 | 6.13 | 5.39 |
| | $^1\Delta_u(\mathrm{V}; \pi \rightarrow \pi^\star)$ | 5.61 | 6.39 | 5.67 |
| | $^3\Sigma_u^+(\mathrm{V}; \pi \rightarrow \pi^\star)$ | 4.10 | 4.54 | 4.13 |
| | $^3\Delta_u(\mathrm{V}; \pi \rightarrow \pi^\star)$ | 4.78 | 5.28 | 4.82 |
| Diazomethane | $^1A_2(\mathrm{V}; \pi \rightarrow \pi^\star)$ | 3.14 | 3.27 | 3.13 |
| | $^1B_1(\mathrm{R}; \pi \rightarrow 3s)$ | 5.54 | 4.59 | 5.57 |
| | $^1A_1(\mathrm{V}; \pi \rightarrow \pi^\star)$ | 5.90 | 5.65 | 6.28 |
| | $^3A_2(\mathrm{V}; \pi \rightarrow \pi^\star)$ | 2.79 | 3.02 | 2.88 |
| | $^3A_1(\mathrm{V}; \pi \rightarrow \pi^\star)$ | 4.05 | 4.27 | 4.12 |
| | $^3B_1(\mathrm{R}; \pi \rightarrow 3s)$ | 5.35 | 4.45 | 5.42 |
| | $^3A_1(\mathrm{R}; \pi \rightarrow 3p)$ | 6.82 | 6.34 | 7.02 |
| | $^1A''[\mathrm{F}](\mathrm{V}; \pi \rightarrow \pi^\star)$ | 0.71 | 0.72 | 0.68 |
| Formamide | $^1A''(\mathrm{V}; n \rightarrow \pi^\star)$ | 5.65 | 5.95 | 5.73 |
| | $^1A'(\mathrm{R}; n \rightarrow 3s)$ | 6.77 | 6.17 | 6.92 |
| | $^1A'(\mathrm{R}; n \rightarrow 3p)$ | *7.38* | 6.74 | 7.57 |
| | $^1A'(\mathrm{V}; \pi \rightarrow \pi^\star)$ | *7.63* | 8.80 | 8.11 |
| | $^3A''(\mathrm{V}; n \rightarrow \pi^\star)$ | 5.38 | 5.89 | 5.44 |
| | $^3A'(\mathrm{V}; \pi \rightarrow \pi^\star)$ | 5.81 | 6.10 | 5.98 |
| Furan | $^1A_2(\mathrm{R}; \pi \rightarrow 3s)$ | 6.09 | 5.26 | 6.27 |
| | $^1B_2(\mathrm{V}; \pi \rightarrow \pi^\star)$ | 6.37 | 7.78 | 6.43 |
| | $^1A_1(\mathrm{V}; \pi \rightarrow \pi^\star)$ | 6.56 | 6.73 | 6.83 |
| | $^1B_1(\mathrm{R}; \pi \rightarrow 3p)$ | 6.64 | 6.07 | 6.72 |
| | $^1A_2(\mathrm{R}; \pi \rightarrow 3p)$ | 6.81 | 5.87 | 6.98 |
| | $^1B_2(\mathrm{R}; \pi \rightarrow 3p)$ | 7.24 | 6.54 | 7.06 |
| | $^3B_2(\mathrm{V}; \pi \rightarrow \pi^\star)$ | 4.20 | 3.94 | 4.43 |
| | $^3A_1(\mathrm{V}; \pi \rightarrow \pi^\star)$ | 5.46 | 5.41 | 5.63 |
| | $^3A_2(\mathrm{R}; \pi \rightarrow 3s)$ | 6.02 | 5.57 | 6.09 |
| | $^3B_1(\mathrm{R}; \pi \rightarrow 3p)$ | 6.59 | 6.04 | 6.68 |
| Glyoxal | $^1A_u(\mathrm{V}; n \rightarrow \pi^\star)$ | 2.88 | 3.42 | 2.99 |
| | $^1B_g(\mathrm{V}; n \rightarrow \pi^\star)$ | 4.24 | 4.68 | 4.38 |
| | $^1A_g(\mathrm{V}; n, n \rightarrow \pi^\star, \pi^\star)$ | 5.61 | 5.92 | 5.55 |
| | $^1B_g(\mathrm{V}; n \rightarrow \pi^\star)$ | 6.57 | 7.35 | 6.80 |
| | $^1B_u(\mathrm{R}; n \rightarrow 3p)$ | 7.71 | 7.04 | 7.81 |
| | $^3A_u(\mathrm{V}; n \rightarrow \pi^\star)$ | 2.49 | 3.06 | 2.59 |
| | $^3B_g(\mathrm{V}; n \rightarrow \pi^\star)$ | 3.89 | 4.61 | 4.10 |
| | $^3B_u(\mathrm{V}; \pi \rightarrow \pi^\star)$ | 5.15 | 5.46 | 5.21 |
| | $^3A_g(\mathrm{V}; \pi \rightarrow \pi^\star)$ | 6.30 | 6.69 | 6.41 |
| Imidazole | $^1A''(\mathrm{R}; \pi \rightarrow 3s)$ | 5.70 | 5.04 | 5.92 |
| | $^1A'(\mathrm{R}; \pi \rightarrow 3p)$ | 6.41 | 6.18 | 6.77 |
| | $^1A''(\mathrm{R}; \pi \rightarrow 3p)$ | 6.50 | 5.43 | 6.80 |
| | $^1A''(\mathrm{V}; n \rightarrow \pi^\star)$ | 6.71 | 7.13 | 7.01 |
| | $^1A'(\mathrm{V}; \pi \rightarrow \pi^\star)$ | 6.86 | 6.73 | 7.06 |
| | $^1A'(\mathrm{R}; n \rightarrow 3s)$ | 7.00 | 6.36 | 7.20 |
| | $^3A'(\mathrm{V}; \pi \rightarrow \pi^\star)$ | 4.74 | 4.55 | 4.88 |
| | $^3A''(\mathrm{R}; \pi \rightarrow 3s)$ | 5.66 | 5.03 | 5.90 |
| | $^3A'(\mathrm{V}; \pi \rightarrow \pi^\star)$ | 5.74 | 5.69 | 5.96 |
| | $^3A''(\mathrm{V}; n \rightarrow \pi^\star)$ | 6.31 | 6.58 | 6.51 |

[a] Significant double excitation character.

Table S14: Comparisons between theoretical best estimates (TBEs) obtained with *aug*-cc-pVTZ and VTEs obtained at the CASSCF (CAS) and SC-NEVPT2 (SC-NEV) levels of theory. See caption of Table S13 for details.

| Compound | State | TBE | CAS | SCNEV |
|---|---|---|---|---|
| Isobutene | $^1B_1(\mathrm{R}; \pi \rightarrow 3s)$ | 6.46 | 6.21 | 6.66 |
| | $^1A_1(\mathrm{R}; \pi \rightarrow 3p)$ | 7.01 | 6.90 | 7.25 |
| | $^3A_1(\mathrm{V}; \pi \rightarrow \pi^\star)$ | 4.53 | 4.66 | 4.61 |
| Ketene | $^1A_2(\mathrm{V}; \pi \rightarrow \pi^\star)$ | 3.86 | 3.98 | 3.97 |
| | $^1B_1(\mathrm{R}; \pi \rightarrow 3s)$ | 6.01 | 5.22 | 6.07 |
| | $^1A_2(\mathrm{R}; \pi \rightarrow 3p)$ | 7.18 | 6.38 | 7.26 |
| | $^3A_2(\mathrm{V}; \pi \rightarrow \pi^\star)$ | 3.77 | 3.92 | 3.85 |
| | $^3A_1(\mathrm{V}; \pi \rightarrow \pi^\star)$ | 5.61 | 5.79 | 5.69 |
| | $^3B_1(\mathrm{R}; \pi \rightarrow 3s)$ | 5.79 | 5.05 | 5.87 |
| | $^3A_2(\mathrm{R}; \pi \rightarrow 3p)$ | 7.12 | 6.35 | 7.22 |
| | $^1A''[\mathrm{F}](\mathrm{V}; \pi \rightarrow \pi^\star)$ | 1.00 | 0.95 | 1.04 |
| Methylenecyclopropene | $^1B_2(\mathrm{V}; \pi \rightarrow \pi^\star)$ | 4.28 | 4.47 | 4.40 |
| | $^1B_1(\mathrm{R}; \pi \rightarrow 3s)$ | 5.44 | 4.92 | 5.49 |
| | $^1A_2(\mathrm{R}; \pi \rightarrow 3p)$ | 5.96 | 5.37 | 6.00 |
| | $^1A_1(\mathrm{V}; \pi \rightarrow \pi^\star)$ | *6.12* | 5.37 | 6.37 |
| | $^3B_2(\mathrm{V}; \pi \rightarrow \pi^\star)$ | 3.49 | 3.44 | 3.67 |
| | $^3A_1(\mathrm{V}; \pi \rightarrow \pi^\star)$ | 4.74 | 4.60 | 4.89 |
| Nitrosomethane | $^1A''(\mathrm{V}; n \rightarrow \pi^\star)$ | 1.96 | 2.12 | 1.95 |
| | $^1A'(\mathrm{V}; n, n \rightarrow \pi^\star, \pi^\star)$ | 4.76 | 4.74 | 4.73 |
| | $^1A'(\mathrm{R}; n \rightarrow 3s)$ | 6.29 | 5.87 | 6.38 |
| | $^3A''(\mathrm{V}; n \rightarrow \pi^\star)$ | 1.16 | 1.31 | 1.13 |
| | $^3A'(\mathrm{V}; \pi \rightarrow \pi^\star)$ | 5.60 | 5.52 | 5.54 |
| | $^1A''[\mathrm{F}](\mathrm{V}; n \rightarrow \pi^\star)$ | 1.67 | 1.83 | 1.66 |
| Propynal | $^1A''(\mathrm{V}; n \rightarrow \pi^\star)$ | 3.80 | 4.00 | 3.98 |
| | $^1A''(\mathrm{V}; \pi \rightarrow \pi^\star)$ | 5.54 | 6.62 | 5.58 |
| | $^3A''(\mathrm{V}; n \rightarrow \pi^\star)$ | 3.47 | 3.52 | 3.61 |
| | $^3A'(\mathrm{V}; \pi \rightarrow \pi^\star)$ | 4.47 | 4.69 | 4.66 |
| Pyrazine | $^1B_{3u}(\mathrm{V}; n \rightarrow \pi^\star)$ | 4.15 | 4.76 | 4.22 |
| | $^1A_u(\mathrm{V}; n \rightarrow \pi^\star)$ | 4.98 | 5.90 | 4.82 |
| | $^1B_{2u}(\mathrm{V}; \pi \rightarrow \pi^\star)$ | 5.02 | 4.97 | 5.36 |
| | $^1B_{2g}(\mathrm{V}; n \rightarrow \pi^\star)$ | 5.71 | 5.80 | 5.92 |
| | $^1A_g(\mathrm{R}; n \rightarrow 3s)$ | 6.65 | 6.69 | 6.73 |
| | $^1B_{1g}(\mathrm{V}; n \rightarrow \pi^\star)$ | 6.74 | 7.16 | 6.80 |
| | $^1B_{1u}(\mathrm{V}; \pi \rightarrow \pi^\star)$ | 6.88 | 8.04 | 6.89 |
| | $^1B_{1g}(\mathrm{R}; \pi \rightarrow 3s)$ | 7.21 | 6.73 | 7.33 |
| | $^1B_{2u}(\mathrm{R}; n \rightarrow 3p)$ | 7.24 | 7.49 | 7.29 |
| | $^1B_{1u}(\mathrm{R}; n \rightarrow 3p)$ | 7.44 | 7.83 | 7.49 |
| | $^1B_{1u}(\mathrm{V}; \pi \rightarrow \pi^\star)$ | *7.98* | 9.65 | 8.42 |
| | $^3B_{3u}(\mathrm{V}; n \rightarrow \pi^\star)$ | 3.59 | 4.16 | 3.61 |
| | $^3B_{1u}(\mathrm{V}; \pi \rightarrow \pi^\star)$ | 4.35 | 3.98 | 4.58 |
| | $^3B_{2u}(\mathrm{V}; (\pi \rightarrow \pi^\star)$ | 4.39 | 4.62 | 4.46 |
| | $^3A_u(\mathrm{V}; n \rightarrow \pi^\star)$ | 4.93 | 5.85 | 4.80 |
| | $^3B_{2g}(\mathrm{V}; n \rightarrow \pi^\star)$ | 5.08 | 5.25 | 5.25 |
| | $^3B_{1u}(\mathrm{V}; \pi \rightarrow \pi^\star)$ | 5.28 | 5.15 | 5.37 |
| Pyridazine | $^1B_1(\mathrm{V}; n \rightarrow \pi^\star)$ | 3.83 | 4.29 | 3.84 |
| | $^1A_2(\mathrm{V}; n \rightarrow \pi^\star)$ | 4.37 | 4.83 | 4.44 |
| | $^1A_1(\mathrm{V}; \pi \rightarrow \pi^\star)$ | 5.26 | 5.12 | 5.61 |
| | $^1A_2(\mathrm{V}; n \rightarrow \pi^\star)$ | 5.72 | 6.26 | 5.95 |
| | $^1B_2(\mathrm{R}; n \rightarrow 3s)$ | 6.17 | 5.99 | 6.23 |
| | $^1B_1(\mathrm{V}; n \rightarrow \pi^\star)$ | 6.37 | 7.16 | 6.71 |
| | $^1B_2(\mathrm{V}; \pi \rightarrow \pi^\star)$ | 6.75 | 7.58 | 7.20 |
| | $^3B_1(\mathrm{V}; n \rightarrow \pi^\star)$ | 3.19 | 3.60 | 3.17 |
| | $^3A_2(\mathrm{V}; n \rightarrow \pi^\star)$ | 4.11 | 4.49 | 4.17 |
| | $^3B_2(\mathrm{V}; \pi \rightarrow \pi^\star)$ | *4.34* | 4.06 | 4.51 |
| | $^3A_1(\mathrm{V}; \pi \rightarrow \pi^\star)$ | 4.82 | 4.93 | 4.97 |
| Pyridine | $^1B_1(\mathrm{V}; n \rightarrow \pi^\star)$ | 4.95 | 5.43 | 5.19 |
| | $^1B_2(\mathrm{V}; \pi \rightarrow \pi^\star)$ | 5.14 | 5.03 | 5.34 |
| | $^1A_2(\mathrm{V}; n \rightarrow \pi^\star)$ | 5.40 | 6.30 | 5.35 |
| | $^1A_1(\mathrm{V}; \pi \rightarrow \pi^\star)$ | 6.62 | 7.90 | 6.80 |
| | $^1A_1(\mathrm{R}; n \rightarrow 3s)$ | 6.76 | 6.40 | 7.00 |
| | $^1A_2(\mathrm{R}; \pi \rightarrow 3s)$ | 6.82 | 6.60 | 6.89 |
| | $^1B_2(\mathrm{V}; \pi \rightarrow \pi^\star)$ | *7.40* | 7.45 | 7.88 |
| | $^1B_1(\mathrm{R}; \pi \rightarrow 3p)$ | 7.38 | 7.12 | 7.47 |
| | $^1A_1(\mathrm{V}; \pi \rightarrow \pi^\star)$ | 7.39 | 9.49 | 7.31 |
| | $^3A_1(\mathrm{V}; \pi \rightarrow \pi^\star)$ | 4.30 | 3.98 | 4.62 |
| | $^3B_1(\mathrm{V}; n \rightarrow \pi^\star)$ | 4.46 | 4.65 | 4.60 |
| | $^3B_2(\mathrm{V}; \pi \rightarrow \pi^\star)$ | 4.79 | 4.83 | 4.91 |
| | $^3A_1(\mathrm{V}; \pi \rightarrow \pi^\star)$ | 5.04 | 5.11 | 5.22 |
| | $^3A_2(\mathrm{V}; n \rightarrow \pi^\star)$ | 5.36 | 5.94 | 5.37 |
| | $^3B_2(\mathrm{V}; \pi \rightarrow \pi^\star)$ | 6.24 | 6.93 | 6.37 |
| Pyrimidine | $^1B_1(\mathrm{V}; n \rightarrow \pi^\star)$ | 4.44 | 4.85 | 4.60 |
| | $^1A_2(\mathrm{V}; n \rightarrow \pi^\star)$ | 4.85 | 5.52 | 4.90 |
| | $^1B_2(\mathrm{V}; \pi \rightarrow \pi^\star)$ | 5.38 | 5.23 | 5.55 |
| | $^1A_2(\mathrm{V}; n \rightarrow \pi^\star)$ | 5.92 | 6.70 | 6.10 |
| | $^1B_1(\mathrm{V}; n \rightarrow \pi^\star)$ | 6.26 | 7.20 | 6.49 |
| | $^1B_2(\mathrm{R}; n \rightarrow 3s)$ | 6.70 | 6.86 | 6.83 |
| | $^1A_1(\mathrm{V}; \pi \rightarrow \pi^\star)$ | 6.88 | 7.62 | 7.21 |
| | $^3B_1(\mathrm{V}; n \rightarrow \pi^\star)$ | 4.09 | 4.45 | 4.21 |
| | $^3A_1(\mathrm{V}; \pi \rightarrow \pi^\star)$ | *4.51* | 4.25 | 4.68 |
| | $^3A_2(\mathrm{V}; n \rightarrow \pi^\star)$ | 4.66 | 5.20 | 4.76 |
| | $^3B_2(\mathrm{V}; \pi \rightarrow \pi^\star)$ | 4.96 | 5.00 | 5.05 |
| Pyrrole | $^1A_2(\mathrm{R}; \pi \rightarrow 3s)$ | 5.24 | 4.49 | 5.51 |
| | $^1B_1(\mathrm{R}; \pi \rightarrow 3p)$ | 6.00 | 5.22 | 6.31 |
| | $^1A_2(\mathrm{R}; \pi \rightarrow 3p)$ | 6.00 | 4.89 | 6.42 |
| | $^1B_2(\mathrm{V}; (\pi \rightarrow \pi^\star)$ | 6.26 | 7.73 | 6.71 |
| | $^1A_1(\mathrm{V}; \pi \rightarrow \pi^\star)$ | 6.30 | 6.47 | 6.58 |
| | $^1B_2(\mathrm{R}; \pi \rightarrow 3p)$ | 6.83 | 5.82 | 6.65 |
| | $^3B_2(\mathrm{V}; \pi \rightarrow \pi^\star)$ | 4.51 | 4.24 | 4.76 |
| | $^3A_2(\mathrm{R}; \pi \rightarrow 3s)$ | 5.21 | 4.47 | 5.48 |
| | $^3A_1(\mathrm{V}; \pi \rightarrow \pi^\star)$ | 5.45 | 5.52 | 5.60 |
| | $^3B_1(\mathrm{R}; \pi \rightarrow 3p)$ | 5.91 | 5.18 | 6.27 |
| Streptocyanine-C1 | $^1B_2(\mathrm{V}; \pi \rightarrow \pi^\star)$ | 7.13 | 7.82 | 7.34 |
| | $^3B_2(\mathrm{V}; \pi \rightarrow \pi^\star)$ | 5.52 | 5.86 | 5.62 |
| Tetrazine | $^1B_{3u}(\mathrm{V}; n \rightarrow \pi^\star)$ | 2.47 | 2.99 | 2.40 |
| | $^1A_u(\mathrm{V}; n \rightarrow \pi^\star)$ | 3.69 | 4.37 | 3.63 |
| | $^1A_g(\mathrm{V}; n, n \rightarrow \pi^\star, \pi^\star)$ | *4.61* | 5.42 | 4.69 |
| | $^1B_{1g}(\mathrm{V}; n \rightarrow \pi^\star)$ | 4.93 | 5.41 | 5.02 |
| | $^1B_{2u}(\mathrm{V}; \pi \rightarrow \pi^\star)$ | 5.21 | 5.04 | 5.60 |
| | $^1B_{2g}(\mathrm{V}; n \rightarrow \pi^\star)$ | 5.45 | 5.43 | 5.68 |
| | $^1A_u(\mathrm{V}; n \rightarrow \pi^\star)$ | 5.53 | 6.37 | 5.70 |
| | $^1B_{3g}(\mathrm{V}; n, n \rightarrow \pi^\star, \pi^\star)$ | *6.15* | 6.59 | 5.70 |
| | $^1B_{2g}(\mathrm{V}; n \rightarrow \pi^\star)$ | 6.12 | 6.79 | 6.21 |
| | $^1B_{1g}(\mathrm{V}; n \rightarrow \pi^\star)$ | 6.91 | 7.18 | 6.83 |
| | $^3B_{3u}(\mathrm{V}; n \rightarrow \pi^\star)$ | 1.85 | 2.38 | 1.78 |
| | $^3A_u(\mathrm{V}; n \rightarrow \pi^\star)$ | 3.45 | 4.06 | 3.41 |
| | $^3B_{1g}(\mathrm{V}; n \rightarrow \pi^\star)$ | 4.20 | 4.66 | 4.29 |
| | $^3B_{1u}(\mathrm{V}; \pi \rightarrow \pi^\star)$ | *4.49* | 3.90 | 4.70 |
| | $^3B_{2u}(\mathrm{V}; \pi \rightarrow \pi^\star)$ | 4.52 | 4.68 | 4.61 |
| | $^3B_{2g}(\mathrm{V}; n \rightarrow \pi^\star)$ | 5.04 | 5.17 | 5.30 |
| | $^3A_u(\mathrm{V}; n \rightarrow \pi^\star)$ | 5.11 | 6.12 | 5.22 |
| | $^3B_{3g}(\mathrm{V}; n, n \rightarrow \pi^\star, \pi^\star)$ | *5.51* | 6.56 | 5.57 |
| | $^3B_{1u}(\mathrm{V}; \pi \rightarrow \pi^\star)$ | 5.42 | 5.32 | 5.59 |

Table S15: Comparisons between theoretical best estimates (TBEs) obtained with *aug*-cc-pVTZ and VTEs obtained at the CASSCF (CAS) and SC-NEVPT2 (SC-NEV) levels of theory. See caption of Table S13 for details.

| Compound | State | TBE | CAS | SCNEV | Compound | State | TBE | CAS | SCNEV |
|---|---|---|---|---|---|---|---|---|---|
| Thioacetone | $^1A_2(\mathrm{V}; n \to \pi^\star)$ | 2.53 | 2.72 | 2.56 | Thiopropynal | $^1A''(\mathrm{V}; n \to \pi^\star)$ | 2.03 | 2.06 | 2.07 |
| | $^1B_2(\mathrm{R}; n \to 4s)$ | 5.56 | 4.80 | 5.69 | | $^3A''(\mathrm{V}; n \to \pi^\star)$ | 1.80 | 1.85 | 1.82 |
| | $^1A_1(\mathrm{V}; \pi \to \pi^\star)$ | 5.88 | 6.94 | 6.38 | Triazine | $^1A_1''(\mathrm{V}; n \to \pi^\star)$ | 4.72 | 5.88 | 4.71 |
| | $^1B_2(\mathrm{R}; n \to 4p)$ | 6.51 | 5.57 | 6.60 | | $^1A_2''(\mathrm{V}; n \to \pi^\star)$ | 4.75 | 5.14 | 4.94 |
| | $^1A_1(\mathrm{R}; n \to 4p)$ | 6.61 | 6.24 | 6.57 | | $^1E''(\mathrm{V}; n \to \pi^\star)$ | 4.78 | 5.51 | 4.94 |
| | $^3A_2(\mathrm{V}; n \to \pi^\star)$ | 2.33 | 2.52 | 2.34 | | $^1A_2'(\mathrm{V}; \pi \to \pi^\star)$ | 5.75 | 5.55 | 5.98 |
| | $^3A_1(\mathrm{V}; \pi \to \pi^\star)$ | 3.45 | 3.52 | 3.48 | | $^1A_1'(\mathrm{V}; \pi \to \pi^\star)$ | 7.24 | 8.20 | 7.42 |
| Thiophene | $^1A_1(\mathrm{V}; \pi \to \pi^\star)$ | 5.64 | 6.11 | 5.92 | | $^1E'(\mathrm{R}; n \to 3s)$ | 7.32 | 7.40 | 7.51 |
| | $^1B_2(\mathrm{V}; \pi \to \pi^\star)$ | 5.98 | 6.94 | 6.20 | | $^1E''(\mathrm{V}; n \to \pi^\star)$ | 7.78 | 8.26 | 8.07 |
| | $^1A_2(\mathrm{R}; \pi \to 3s)$ | 6.14 | 5.70 | 6.20 | | $^1E'(\mathrm{V}; \pi \to \pi^\star)$ | 7.94 | 10.03 | 8.59 |
| | $^1B_1(\mathrm{R}; \pi \to 3p)$ | 6.14 | 6.02 | 6.20 | | $^3A_2''(\mathrm{V}; n \to \pi^\star)$ | 4.33 | 4.74 | 4.55 |
| | $^1A_2(\mathrm{R}; \pi \to 3p)$ | 6.21 | 6.05 | 6.41 | | $^3E''(\mathrm{V}; n \to \pi^\star)$ | 4.51 | 5.14 | 4.66 |
| | $^1B_1(\mathrm{R}; \pi \to 3s)$ | 6.49 | 5.78 | 6.72 | | $^3A_1''(\mathrm{V}; n \to \pi^\star)$ | 4.73 | 5.88 | 4.81 |
| | $^1B_2(\mathrm{R}; \pi \to 3p)$ | 7.29 | 6.80 | 7.29 | | $^3A_1'(\mathrm{V}; \pi \to \pi^\star)$ | 4.85 | 4.46 | 5.06 |
| | $^1A_1(\mathrm{V}; \pi \to \pi^\star)$ | *7.31* | 8.29 | 7.59 | | $^3E'(\mathrm{V}; \pi \to \pi^\star)$ | 5.59 | 5.57 | 5.77 |
| | $^3B_2(\mathrm{V}; \pi \to \pi^\star)$ | 3.92 | 3.68 | 4.15 | | $^3A_2'(\mathrm{V}; \pi \to \pi^\star)$ | 6.62 | 7.70 | 6.47 |
| | $^3A_1(\mathrm{V}; \pi \to \pi^\star)$ | 4.76 | 4.97 | 4.88 | | | | | |
| | $^3B_1(\mathrm{R}; \pi \to 3p)$ | 5.93 | 5.86 | 5.99 | | | | | |
| | $^3A_2(\mathrm{R}; \pi \to 3s)$ | 6.08 | 5.65 | 6.15 | | | | | |

# S5 Scaling cost

Table S16: Formal scaling with system size for selected single- and multi-reference methods where $N$ is the number of basis functions. I and P stand for the iterative and perturbative steps of the calculation, respectively. Note that the cost of the AO-to-MO integral transformation (which scales as $\mathcal{O}(N^5)$ in the general case) is not taken into account. Of course the computational time and ressources needed to perform a specific calculation will depend not only the selected method, molecule, and basis set but also on the selected code, implementation and computational infrastructure. For multi-reference methods, the scaling prefactor depends on the size of the active space.

| Method | Scaling |
|---|---|
| TD-DFT | I-$\mathcal{O}(N^4)$ |
| BSE/ev$GW$ | I-$\mathcal{O}(N^4)$ |
| CIS(D) | I-$\mathcal{O}(N^4)$+P-$\mathcal{O}(N^5)$ |
| CC2 | I-$\mathcal{O}(N^5)$ |
| ADC(2) | I-$\mathcal{O}(N^5)$ |
| ADC(3) | I-$\mathcal{O}(N^6)$ |
| CCSD | I-$\mathcal{O}(N^6)$ |
| CC3 | I-$\mathcal{O}(N^7)$ |
| NEVPT2 | P-$\mathcal{O}(N^5)$ |
| CASPT2 | P-$\mathcal{O}(N^5)$ |

# References


(1) Loos, P.-F.; Scemama, A.; Blondel, A.; Garniron, Y.; Caffarel, M.; Jacquemin, D. A Mountaineering Strategy to Excited States: Highly-Accurate Reference Energies and Benchmarks. *J. Chem. Theory Comput.* **2018**, *14*, 4360–4379.

(2) Loos, P.-F.; Boggio-Pasqua, M.; Scemama, A.; Caffarel, M.; Jacquemin, D. Reference Energies for Double Excitations. *J. Chem. Theory Comput.* **2019**, *15*, 1939–1956.

(3) Loos, P.-F.; Lipparini, F.; Boggio-Pasqua, M.; Scemama, A.; Jacquemin, D. A Mountaineering Strategy to Excited States: Highly-Accurate Energies and Benchmarks for Medium Size Molecules. *J. Chem. Theory Comput.* **2020**, *16*, 1711–1741.
